# Supplementary material for: Feature Importance Disparities for Data Bias Investigations
Source: arXiv:2303.01704 source file (2024-06-03)
Supplement: Supplementary file 1 [file size_appendix.tex]

\section{Subgroup Sizes Outcomes}
\label{sec:size_app}

In Figure~\ref{fig:size_app} we chart the subgroup sizes, $|g(X_{test})|$, outputted by the algorithms across all dataset and importance notion combinations. As a whole, the final subgroup sizes were generally within the specified $\alpha$ range. Occasionally, there were subgroups which were significantly outside the expected range. Usually this was due to most of the importance values, $F(f_j, X, h)$, being zero for a given feature.

In Figure~\ref{fig:size_gen_app} we compare $|g_j^*(X_{train})|$ and $|g_j^*(X_{test})|$, outputted by the algorithms across all dataset and importance notion combinations. As we can see, the subgroup sizes were very consistent between the train and test set meaning $|g|$ generalized very well. The average difference was only somewhat large on the Student dataset, due to the fact that it is a smaller dataset.

\begin{figure}[H]
\centering
\begin{subfigure}{.3\textwidth}
  \centering
  \includegraphics[width=\linewidth]{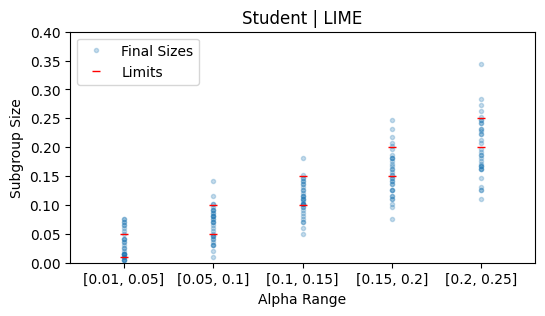}
\end{subfigure}%
\begin{subfigure}{.3\textwidth}
  \centering
  \includegraphics[width=\linewidth]{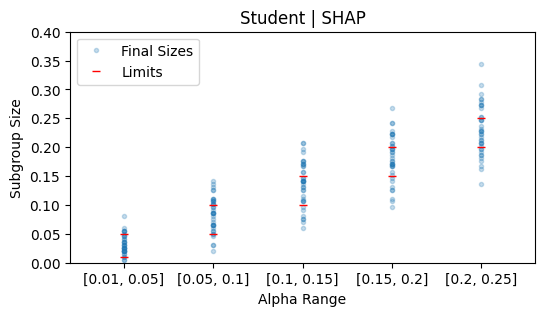}
\end{subfigure}
\begin{subfigure}{.3\textwidth}
  \centering
  \includegraphics[width=\linewidth]{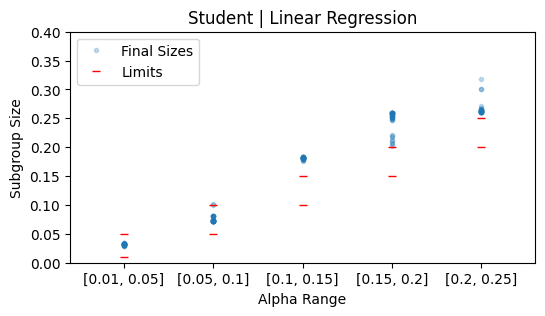}
\end{subfigure} \\

\begin{subfigure}{.3\textwidth}
  \centering
  \includegraphics[width=\linewidth]{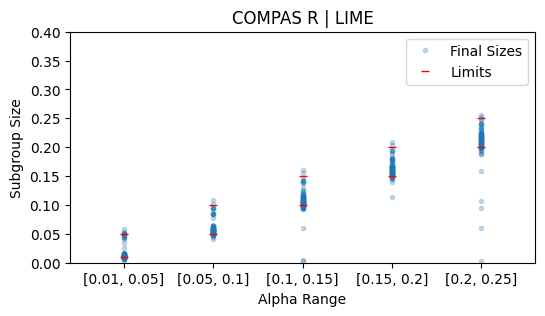}
\end{subfigure}
\begin{subfigure}{.3\textwidth}
  \centering
  \includegraphics[width=\linewidth]{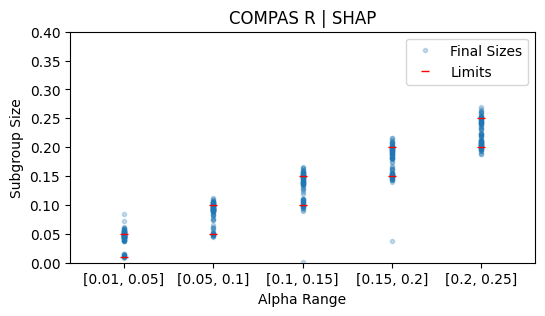}
\end{subfigure}%
\begin{subfigure}{.3\textwidth}
  \centering
  \includegraphics[width=\linewidth]{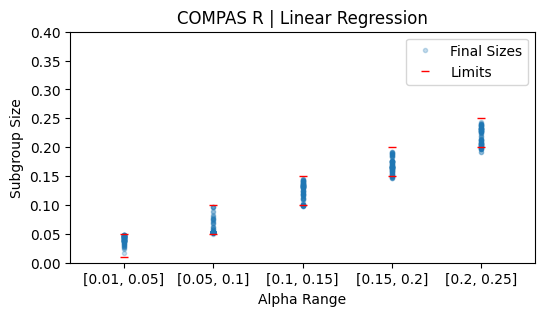}
\end{subfigure} \\

\begin{subfigure}{.3\textwidth}
  \centering
  \includegraphics[width=\linewidth]{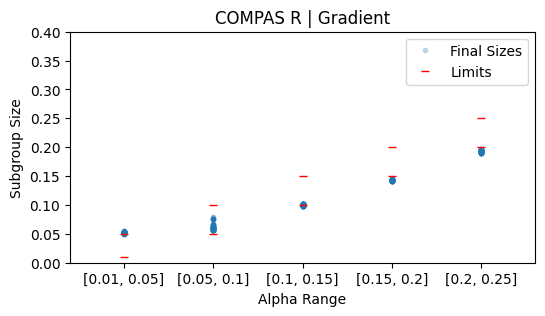}
\end{subfigure}
\begin{subfigure}{.3\textwidth}
  \centering
  \includegraphics[width=\linewidth]{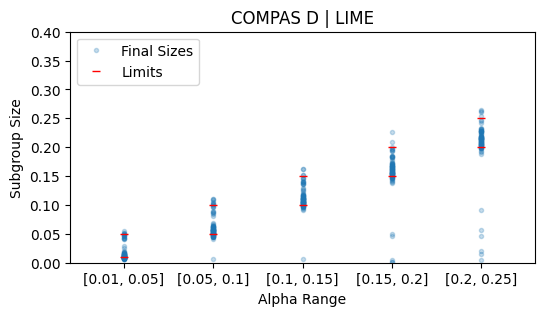}
\end{subfigure}
\begin{subfigure}{.3\textwidth}
  \centering
  \includegraphics[width=\linewidth]{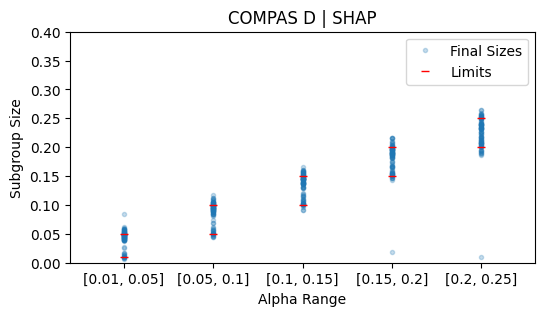}
\end{subfigure} \\

\begin{subfigure}{.3\textwidth}
  \centering
  \includegraphics[width=\linewidth]{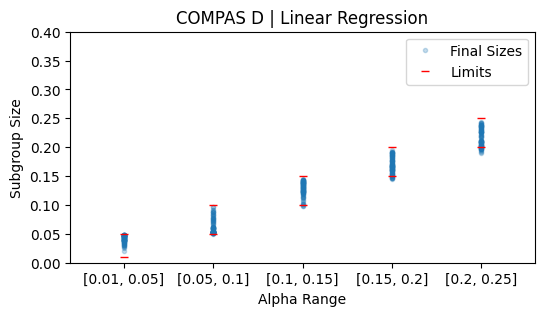}
\end{subfigure}
\begin{subfigure}{.3\textwidth}
  \centering
  \includegraphics[width=\linewidth]{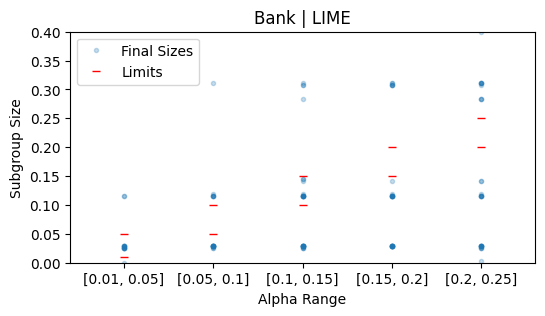}
\end{subfigure}
\begin{subfigure}{.3\textwidth}
  \centering
  \includegraphics[width=\linewidth]{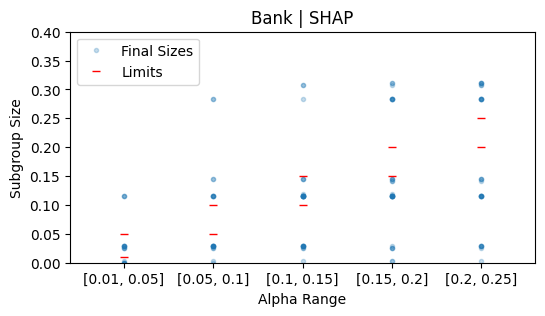}
\end{subfigure} \\

\begin{subfigure}{.3\textwidth}
  \centering
  \includegraphics[width=\linewidth]{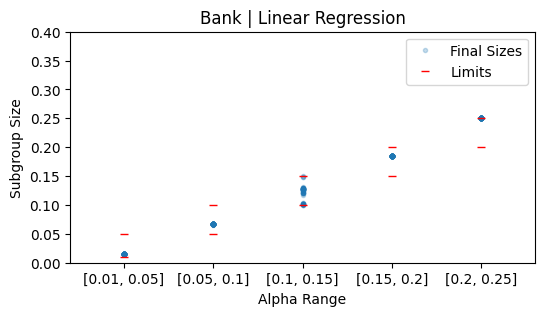}
\end{subfigure}%
\begin{subfigure}{.3\textwidth}
  \centering
  \includegraphics[width=\linewidth]{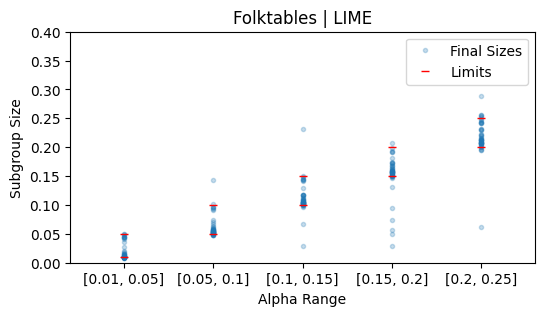}
\end{subfigure}
\begin{subfigure}{.3\textwidth}
  \centering
  \includegraphics[width=\linewidth]{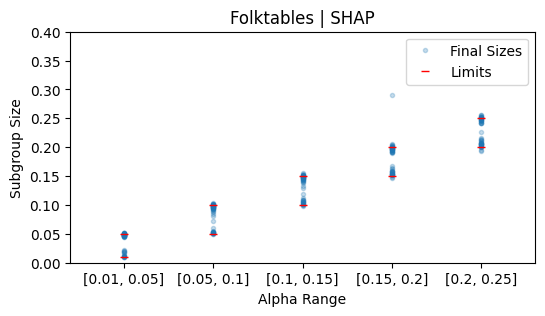}
\end{subfigure} \\

\begin{subfigure}{.3\textwidth}
  \centering
  \includegraphics[width=\linewidth]{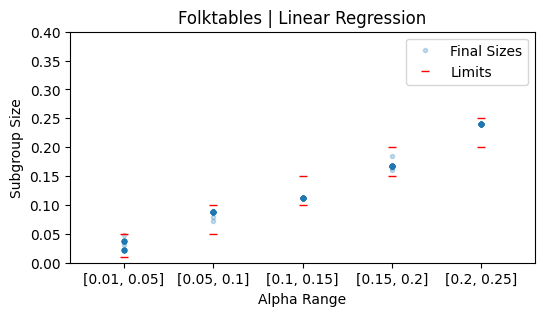}
\end{subfigure}
\caption{Final subgroup sizes of $g(X_{test})$ compared with $\alpha$ range. These almost always fall within the correct size range. Student has the largest errors given the small dataset size. Some subgroups fell significantly outside the expected ranged, mostly due to many importance values, $F(f_j, X, h)$, being zero for a given feature.}
\label{fig:size_app}
\end{figure}

\begin{figure}[H]
\centering
\begin{subfigure}{.245\textwidth}
  \centering
  \includegraphics[width=\linewidth]{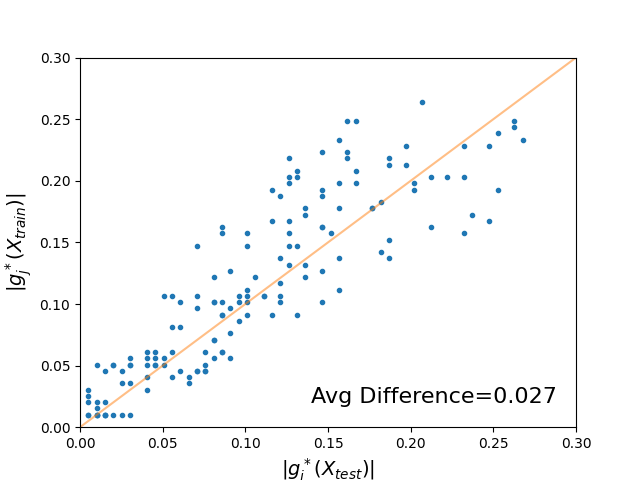}
  \caption{Student, LIME}
\end{subfigure}%
\begin{subfigure}{.245\textwidth}
  \centering
  \includegraphics[width=\linewidth]{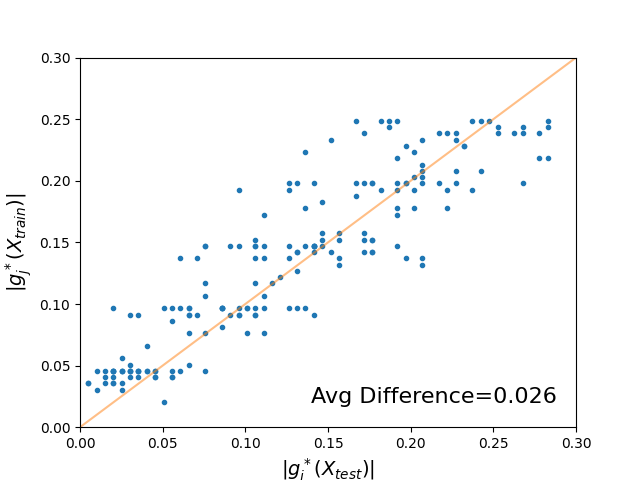}
  \caption{Student, SHAP}
\end{subfigure}
\begin{subfigure}{.245\textwidth}
  \centering
  \includegraphics[width=\linewidth]{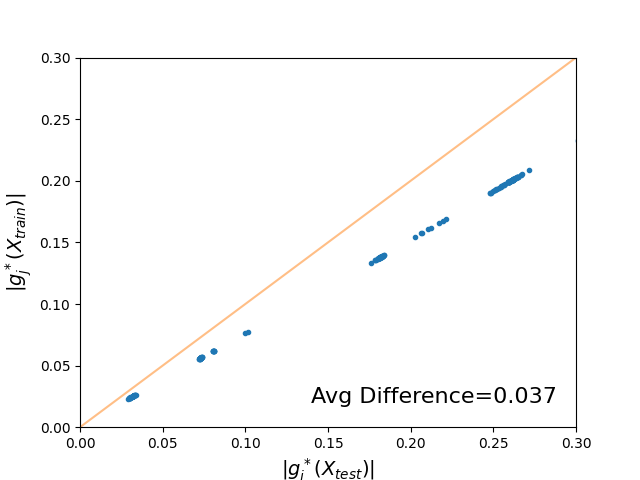}
  \caption{Student, LR}
\end{subfigure}
\begin{subfigure}{.245\textwidth}
  \centering
  \includegraphics[width=\linewidth]{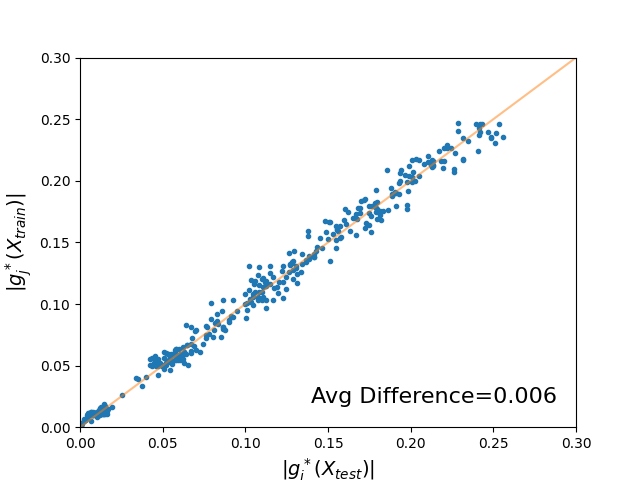}
  \caption{COMPAS R, LIME}
\end{subfigure} \\

\begin{subfigure}{.245\textwidth}
  \centering
  \includegraphics[width=\linewidth]{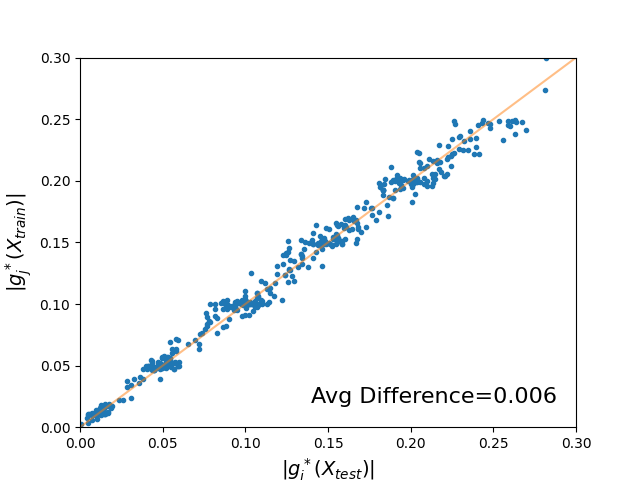}
  \caption{COMPAS R, SHAP}
\end{subfigure}%
\begin{subfigure}{.245\textwidth}
  \centering
  \includegraphics[width=\linewidth]{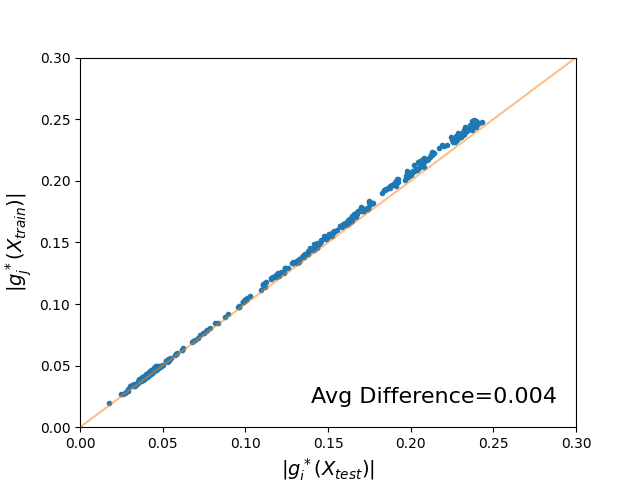}
  \caption{COMPAS R, LR}
\end{subfigure}
\begin{subfigure}{.245\textwidth}
  \centering
  \includegraphics[width=\linewidth]{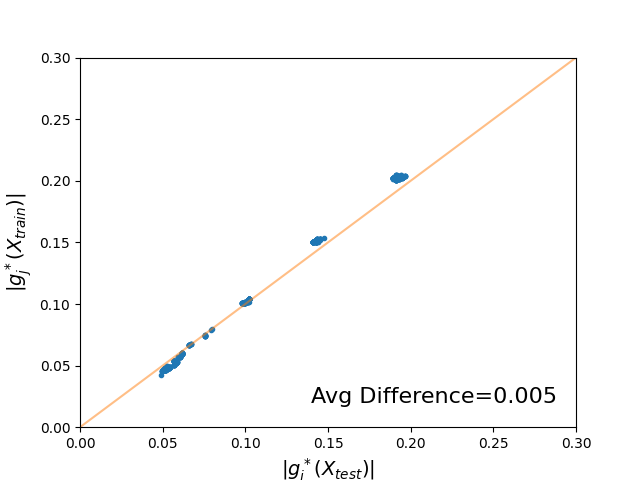}
  \caption{COMPAS R, GRAD}
\end{subfigure}
\begin{subfigure}{.245\textwidth}
  \centering
  \includegraphics[width=\linewidth]{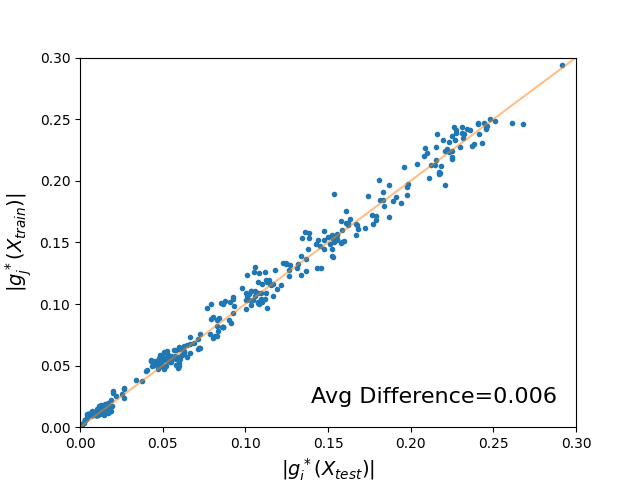}
  \caption{COMPAS D, LIME}
\end{subfigure} \\

\begin{subfigure}{.245\textwidth}
  \centering
  \includegraphics[width=\linewidth]{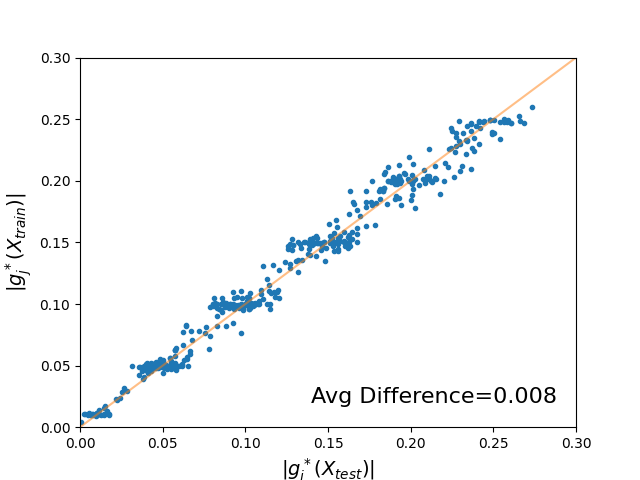}
  \caption{COMPAS D, SHAP}
\end{subfigure}%
\begin{subfigure}{.245\textwidth}
  \centering
  \includegraphics[width=\linewidth]{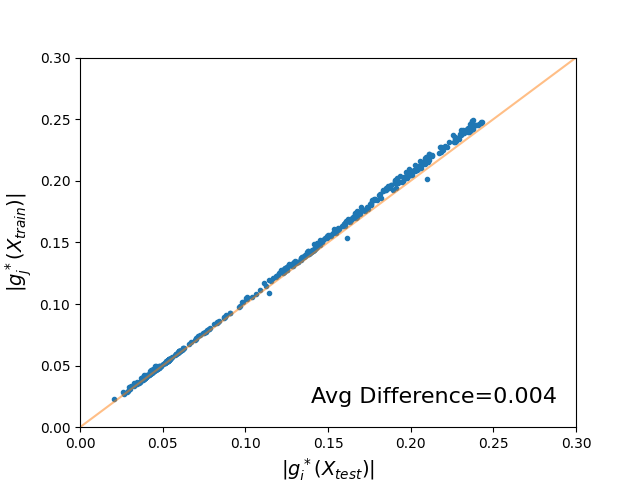}
  \caption{COMPAS D, LR}
\end{subfigure}
\begin{subfigure}{.245\textwidth}
  \centering
  \includegraphics[width=\linewidth]{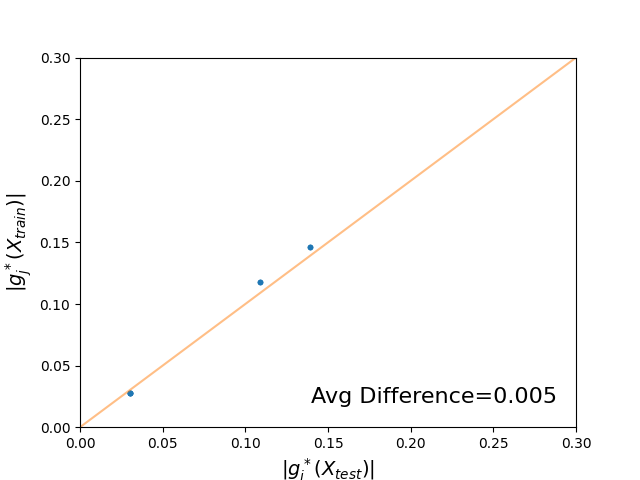}
  \caption{Bank, LIME}
\end{subfigure}
\begin{subfigure}{.245\textwidth}
  \centering
  \includegraphics[width=\linewidth]{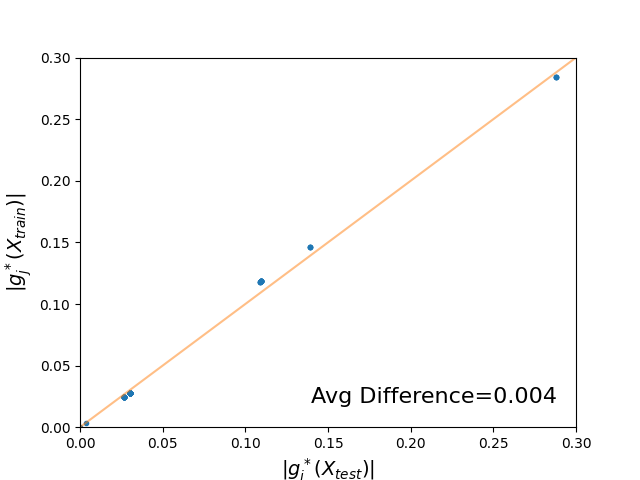}
  \caption{Bank, SHAP}
\end{subfigure} \\

\begin{subfigure}{.245\textwidth}
  \centering
  \includegraphics[width=\linewidth]{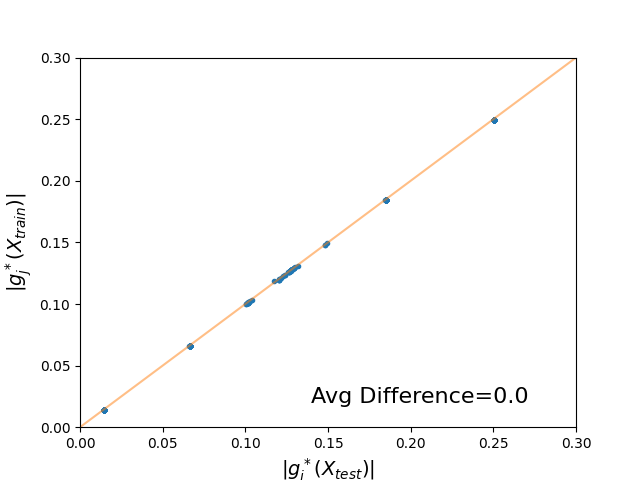}
  \caption{Bank, LR}
\end{subfigure}%
\begin{subfigure}{.245\textwidth}
  \centering
  \includegraphics[width=\linewidth]{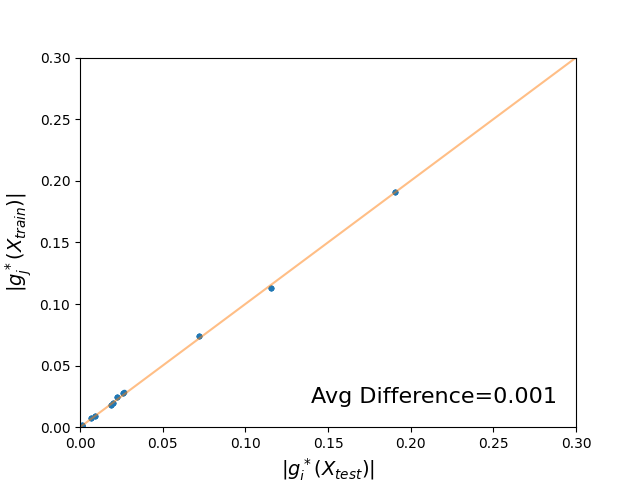}
  \caption{Folk, LIME}
\end{subfigure}
\begin{subfigure}{.245\textwidth}
  \centering
  \includegraphics[width=\linewidth]{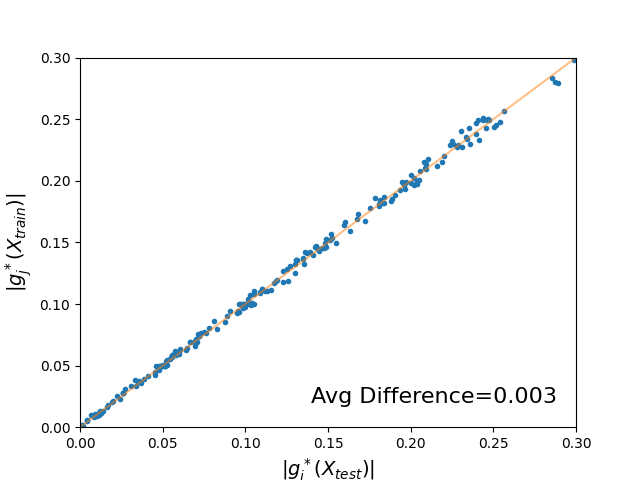}
  \caption{Folk, SHAP}
\end{subfigure}
\begin{subfigure}{.245\textwidth}
  \centering
  \includegraphics[width=\linewidth]{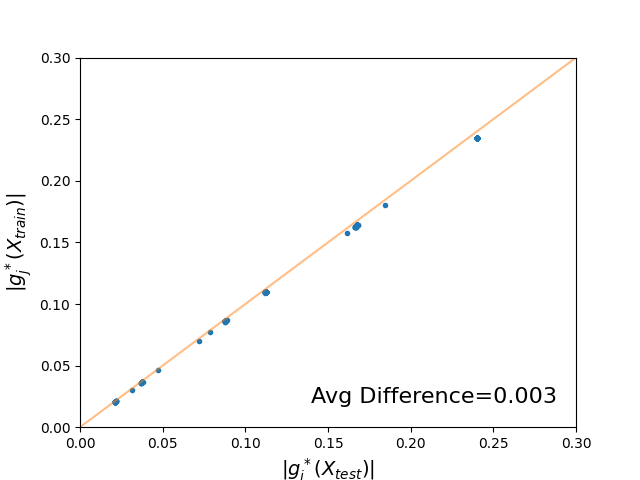}
  \caption{Folk, LR}
\end{subfigure} \\
\caption{Comparing $|g_j^*(X_{train})|$ and $|g_j^*(X_{test})|$. We can see that the size of the subgroup was consistent between the train and test set showing good generalization. The average difference was only noticeable on the Student dataset, due to its smaller size.}
\label{fig:size_gen_app}
\end{figure}
